# Supplementary material for: Reward Augmentation in Reinforcement Learning for Testing Distributed Systems
Source: arXiv:2409.02137 source file (2024-09-02)
Supplement: Supplementary file 1 [file appendix.tex]

\section{Implementation details}

A generic RL exploration requires an environment to query the state, actions and determine the next state after an action. We define a generic interface \texttt{Environment} in our implementation with the following functions,

\begin{lstlisting}[language=Golang]
type Environment interface {
    Reset() State
    Step(Action) State
}

type State interface {
    Actions() Action
}
\end{lstlisting}
    
The \texttt{Reset} method of the environment returns the initial \texttt{State} of the environment. Given a \texttt{State}, the \texttt{Actions} method returns the set of possible actions and the \texttt{Step} method returns the next state as a result of the action. The state space we model for distributed protocols however extends the \texttt{Environment} interface and is still generic to different protocols. Therefore, we define an abstract implementation \texttt{PartitionedEnvironment} that constructs the state and actions as defined in our transition system. In order to test, the developer needs to wrap the implementation with a shim. The shim should extend the abstract interface \texttt{PartitionedEnvironment} as defined below,

\begin{lstlisting}[language=Golang]
type PartitionedEnvironment interface {
    Reset() PartitionState
    Tick() PartitionState
    DeliverMessages([]Message) PartitionState
    DropMessages([]Message) PartitionState
    StartProcess(int) PartitionState
    StopProcess(int) PartitionState
    ReceiveRequest(Request) PartitionState
}

type PartitionState interface {
    GetProcessState(ProcessID) ProcessState
    GetPendingMessages() []Message
    GetPendingRequests() []Request
    CanDeliverRequest() bool
}
\end{lstlisting}

Note that the methods of \texttt{PartitionedEnvironment} return a \texttt{PartitionState} that we use to construct the \texttt{State} object for RL. Additionally, the methods correspond to enacting specific actions. \texttt{DeliverMessages} and \texttt{DropMessages} are used when the action is to move to a different partition configuration. \texttt{StartProcess} and \texttt{StopProcess} are invoked when we handle the crash and start actions. Finally, \texttt{ReceiveRequest} is used when handling the action to inject a request to the system.

The missing detail so far is the mechanism to introduce a color abstraction. We introduce a generic \texttt{Painter} interface to abstract the local state of each process (represented by \texttt{ProcessState}).

\begin{lstlisting}[language=Golang]
type Painter interface {
    ColorState(ProcessState) Color
}
\end{lstlisting}

In our implementation, we define a generic predicate with boolean connectives as a follows,
\begin{lstlisting}[language=Golang]
type Predicate func(State) bool

func (p Predicate) And(o Predicate) Predicate
func (p Predicate) Or(o Predicate) Predicate
func (p Predicate) Not() Predicate
\end{lstlisting}

\section{Statistical significance test}
\label{sec:statistical_tests}
We list the values for the non parametric Mann Whitney U statistical test. The test determines if two samples are from different statistical distributions. The test outputs a value which if $>0.05$ then we reject the hypothesis. We report the test values in Table~\ref{tab:results_stat_test} for all the target predicates where we compare \biasExpAlgo{} vs other pure exploration approaches.

\begin{table}[]
	\centering
	\small
	\begin{tabular}{|l|c|c|c|}
		\toprule
		Benchmarks            & BonusMaxRL       & NegRLVisits      & Random           \\
		\midrule
		\textbf{RedisRaft} & & & \\
		OneInTerm3            &      0.70            &      0.86            &     0.01             \\
		AllInTerm2            &      8.25e-06            &      8.25e-06           &     8.22e-06             \\
		TermDiff2             &      0.14            &      0.40            &     4.46e-03             \\
		CommitEntries2        &      8.25e-06            &      8.25e-06            &     8.25e-06             \\
		EntryInTerm2          &      8.25e-06            &      8.25e-06            &     8.25e-06            \\
		LeaderInTerm2         &      8.25e-06            &      8.25e-06           &     8.25e-06             \\
		LogDiff1              &      8.25e-06            &      8.25e-06            &     8.25e-06             \\
		LogCommitDiff3        &      1.25e-05            &      1.25e-05            &     1.25e-05             \\
		OneLeaderOneCandidate &      6.91e-03          &      5.17e-03            &     9.07e-05             \\
		\hline
		\textbf{Etcd} & & & \\
		LogCommitGap3 & 9.13e-05 & 9.13e-05 & 9.13e-05 \\
        OneInTerm4 & 9.13e-05 & 9.13e-05 & 9.13e-05 \\
        MinCommit2 & 9.13e-05 & 9.13e-05 & 9.08e-05 \\
        TermDiff2 & 9.13e-05 & 9.13e-05 & 9.13e-05 \\
        LeaderInTerm4 & 9.13e-05 & 9.13e-05 & 9.13e-05 \\
        AtLeastOneCommitInTerm2 & 9.13e-05 & 9.13e-05 & 9.13e-05 \\
        OneLeaderOneCandidate & 0.98 & 9.13e-05 & 9.13e-05 \\
        LogGap2 & 2.91e-04 & 0.01 & 9.13e-05 \\
        AllInTerm5 & 1.40e-03 & 1.41e-03 & 9.13e-05 \\
		\hline
		\textbf{RSL} & & & \\
        AnyBallot3 & 9.08e-05 & 9.03e-05 & 9.08e-05 \\
        AllBallot3 & 9.13e-05 & 9.13e-05 & 9.08e-05 \\
        EntryBallot2 & 0.99 & 0.07 & 0.05 \\
        AnyDecree2 & 9.08e-05 & 9.08e-05 & 9.08e-05 \\
        BallotDiff2 & 0.02 & 8.19e-05 & 9.81e-05 \\
        AnyDecided3 & 9.08e-05 & 9.08e-05 & 9.08e-05 \\
        PrimaryInBallot2 & 2.91e-04 & 9.13e-05 & 9.08e-05 \\
		\bottomrule
	\end{tabular}
	\caption{Coverage results for RedisRaft}
	\label{tab:results_stat_test}
\end{table}
